# Supplementary material for: Optimal design of diamond-air microcavities for quantum networks using an analytical approach
Source: arXiv:1806.11474 ancillary file (2018-11-26)
Supplement: Supplementary file 1 [file Supplement.pdf]

# Supplementary information for: Optimal design of diamond-air microcavities for quantum networks using an analytical approach

## I. RESONANCE CONDITION FOR A DIAMOND-AIR CAVITY

To understand how the partially reflective diamond-air interface influences the cavity system, we first look at the resonance condition in diamond and air separately. For the air gap the diamond-air interface from low ($n_a = 1$) to high ($n_d = 2.41$) refractive index results in a field with an antinode at the interface. From the diamond membrane the reflection coefficient is opposite: the field in diamond has a node at this interface. Naturally, when these cavities are coupled, the electric field at the diamond-air interface has to be continuous. It is thus impossible to satisfy the resonance conditions of the two individual cavities at the same time. The result is that the original modes in diamond and air show anti-crossings [1, 2]. The hybridized cavity resonances are given by [1]:

$$\nu = \frac{c}{2\pi(t_a + n_d t_d)} \left( m\pi - (-1)^m \arcsin\left( \frac{n_d - 1}{n_d + 1} \sin\left( \pi m \frac{t_a - n_d t_d}{t_a + n_d t_d} \right) \right) \right), \tag{1}$$

for an air gap of length $t_a$ and a diamond thickness $t_d$. The resulting spectrum is shown in fig. 1(a). We can distinguish two special cases for these resonant modes: the 'air-like mode', in which the hybridized mode has an antinode at the diamond-air interface, and the 'diamond-like mode' in which there is a node at the interface. They correspond to the values for which the sine term on the right-hand side of the resonant condition vanishes:

$$t_d = m_d \frac{\lambda_0}{2n_d} \quad \text{and} \quad t_a = m_a \frac{\lambda_0}{2}; \qquad \textit{(air-like mode)} \tag{2}$$

$$t_d = (2m_d + 1) \frac{\lambda_0}{4n_d} \quad \text{and} \quad t_a = (2m_a - 1) \frac{\lambda_0}{4}; \qquad \textit{(diamond-like mode)} \tag{3}$$

for any integer $(m_a, m_d)$, and $m = m_a + m_d$, and $\lambda_0 = \nu/c$ the free space wavelength.

We next find the resulting condition on $t_a$ given a diamond thickness $t_d$. The resonance condition for a diamond-air cavity (eq. (1)) is derived from the equation [1]:

$$(1 + n_d) \sin\left( \frac{2\pi}{\lambda_0}(t_a + n_d t_d) \right) = (1 - n_d) \sin\left( \frac{2\pi}{\lambda_0}(t_a - n_d t_d) \right). \tag{4}$$

To find the on-resonance air gap $t_a$ as a function of diamond thickness $t_d$, as in Eq. (9) of the main text, we rewrite this in the following steps:

$$(1 + n_d) \left( \sin(\frac{2\pi}{\lambda_0} t_a) \cos(\frac{2\pi}{\lambda_0} n_d t_d) + \cos(\frac{2\pi}{\lambda_0} t_a) \sin(\frac{2\pi}{\lambda_0} n_d t_d) \right) \tag{5}$$

$$= (1 - n_d) \left( \sin(\frac{2\pi}{\lambda_0} t_a) \cos(\frac{2\pi}{\lambda_0} n_d t_d) - \cos(\frac{2\pi}{\lambda_0} t_a) \sin(\frac{2\pi}{\lambda_0} n_d t_d) \right)$$

$$2n_d \sin(\frac{2\pi}{\lambda_0} t_a) \cos(\frac{2\pi}{\lambda_0} n_d t_d) = -2 \cos(\frac{2\pi}{\lambda_0} t_a) \sin(\frac{2\pi}{\lambda_0} n_d t_d) \tag{6}$$

$$n_d \tan(\frac{2\pi}{\lambda_0} t_a) = -\tan(\frac{2\pi}{\lambda_0} n_d t_d) \tag{7}$$

$$t_a = \frac{\lambda_0}{2\pi} \arctan\left( -\frac{1}{n_d} \tan\left( \frac{2\pi n_d t_d}{\lambda_0} \right) \right) \tag{8}$$

## II. EFFECT OF AR COATING OF THE DIAMOND MEMBRANE

With an AR coating applied to the diamond membrane, the electric field distribution is altered to the situation as shown in fig. 2. In the ideal case the AR coating is a layer of refractive index $n_{AR} = \sqrt{n_d} \approx 1.55$ and thickness $t_{AR} = \lambda_0/(4n_{AR})$. In practice, it can be created for example with $SiO_2$ ($n_{SiO_2} \approx 1.46$) or $Al_2O_3$ ($n_{Al_2O_3} \approx 1.77$) [3, 4].

The resonance condition for a cavity with a non-ideal AR coating with refractive index $n_{AR}$ and a thickness $\lambda_0/(4n_{AR})$ is given by:

$$\nu_{AR} = \frac{c}{2\pi(t_a + t_d n_d)} \left( (m + 1/2)\pi - (-1)^m \arcsin\left( \frac{n_{AR}^2 - n_{air} n_d}{n_{AR}^2 + n_{air} n_d} \cos\left( \pi(m + 1/2) \frac{t_a - n_d t_d}{t_a + n_d t_d} \right) \right) \right). \tag{9}$$

For the ideal AR coating with $n_{AR} = \sqrt{n_{air} n_d}$ the second term on the right-hand-side vanishes, and this reduces to the resonance condition expected for a cavity with a single material of optical length $L = t_a + t_d n_d + \lambda_0/(4n_{AR})n_{AR}$:

$$\nu_{ideal,AR} = \frac{(m+1/2)c}{2(t_a + t_d n_d)} \tag{10}$$

The resonance spectrum for the ideal and non-ideal AR coated diamond-air cavities are compared to the hybridized resonance spectra (eq. (1)) in fig. 1.

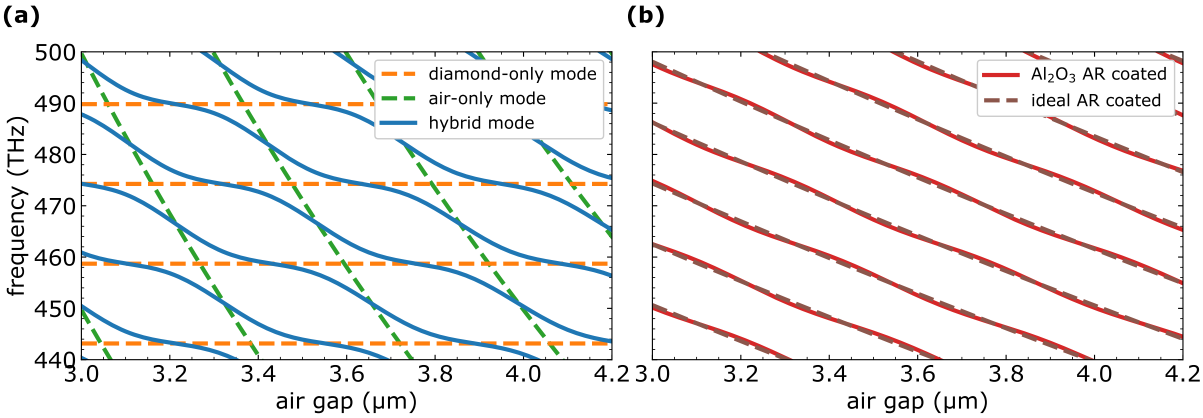


FIG. 1: (a) The diamond-only and air-only resonances follow resonance conditions given by $\nu_d = (2m_d - 1)c/(4n_d t_d)$, and $\nu_a = m_a c/(2t_a)$ with integer $m_d$ and $m_a$ respectively. The frequencies of the resonances of the hybrid cavity are given by eq. (1). (b) With an ideal AR coating with $n_{AR} = \sqrt{n_d}$ the hybrid mode behavior disappears (). An experimental AR coating with $Al_2O_3$ with refractive index $n_{Al_2O_3} = 1.77$ leads to resonance frequencies given by eq. (10) (red solid lines).

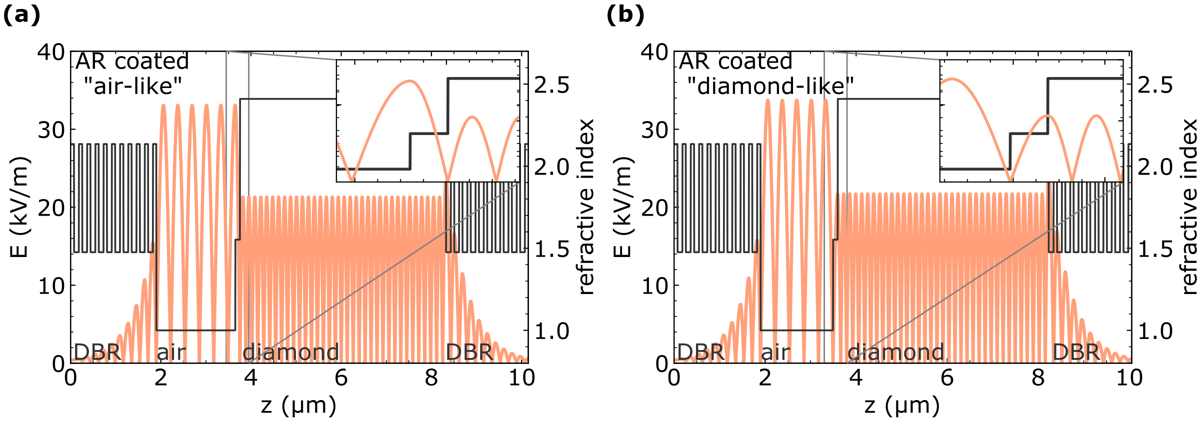


FIG. 2: The electric field distribution for a hybrid cavity with an AR-coated diamond membrane for what would have been (a) an air-like mode (b) a diamond-like mode if there were no AR coating. With this AR coating, the electric field intensity in the diamond and air parts are equal ($E^2_{max,a} = n_d E^2_{max,d}$).

## III. SCATTERING AT A PARTIALLY REFLECTIVE INTERFACE

This section describes how to find the scattering strength for a partially reflective interface.

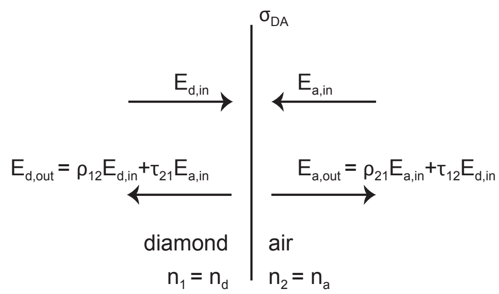


FIG. 3: The losses for a field incident on the diamond air interface are described the difference between the incoming field and the outgoing field for each side of the interface individually, as in eq. (16). The effective total losses in a diamond-air cavity are given by the losses from each side, multiplied by the relative intensity: $\mathcal{L}_{\mathrm{S,eff}} = \mathcal{L}_{DA} + n_a E^2_{max,a}/(n_d E^2_{max,d})\mathcal{L}_{AD}$

Firstly, we define the problem by drawing the schematic in fig. 3. We are going to evaluate the losses upon incidence from the left-hand side and right-hand side individually. Upon incidence, the field can be reflected or transmitted. This can be described by a matching matrix, that is given by [1, 5–8]:

$$\begin{pmatrix} E_{1,in} \\ E_{1,out} \end{pmatrix} = \frac{1}{\tau'_{12}} \begin{pmatrix} 1 & -\rho'_{21} \\ \rho'_{12} & \tau'_{12}\tau'_{21} - \rho'_{12}\rho'_{21} \end{pmatrix} \begin{pmatrix} E_{2,out} \\ E_{2,in} \end{pmatrix}; \tag{11}$$

$$\rho'_{ij} = \rho_{ij} \mathrm{e}^{-2\left(\frac{2\pi\sigma n_i}{\lambda_0}\right)^2} \approx \rho_{ij}\left(1 - 2\left(\frac{2\pi\sigma n_i}{\lambda_0}\right)^2\right);$$

$$\tau'_{ij} = \tau_{ij} \mathrm{e}^{-1/2\left(\frac{2\pi\sigma(n_j - n_i)}{\lambda_0}\right)^2} \approx \tau_{ij}\left(1 - 1/2\left(\frac{2\pi\sigma(n_j - n_i)}{\lambda_0}\right)^2\right); \tag{12}$$

$$\rho_{ij} = \frac{n_i - n_j}{n_i + n_j}; \tag{13}$$

$$\tau_{ij} = \frac{2n_i}{n_i + n_j}.$$

Here $E_{1(2),in}$ and $E_{1(2),out}$ are the incoming and outgoing fields on the left-hand side (right-hand side) of the interface, where the refractive index is $n_1(n_2)$. For the diamond-air interface, we identify $E_{1(2)} = E_{d(a)}$ and $n_1 = n_d$, $n_2 = n_d$. $\rho_{ij}$ and $\tau_{ij}$ are the Fresnel reflection and transmission coefficients, that are extended to $\rho'_{ij}$ and $\tau'_{ij}$ to include scattering at and interface with rms roughness of $\sigma_{ij}$. We use a Taylor expansion to approximate them, keeping only terms up to $\mathrm{O}\left(\left(\frac{2\pi\sigma}{\lambda_0}\right)^2\right)$. Using this formalism, we can write the outgoing fields in terms of the incoming fields as:

$$E_{1,out} = \rho'_{12} E_{1,in} + \tau'_{21} E_{2,in}; \tag{14}$$

$$E_{2,out} = \rho'_{21} E_{2,in} + \tau'_{12} E_{1,in}. \tag{15}$$

The losses from the left side of the interface are described by as the normalised difference between the incoming and outgoing field:

$$\mathcal{L}_{S,12} = \frac{n_1|E_{1,in}|^2 - n_1|E_{1,out}|^2}{n_1|E_{1,in}|^2} \tag{16}$$

$$= 1 - \frac{|\rho'_{12}E_{1,in} + \tau'_{21}E_{2,in}|^2}{|E_{1,in}|^2}, \tag{17}$$

and a similar formulation holds for the right hand side, replacing $1 \leftrightarrow 2$. We see that here the interference between the reflected and transmitted fields plays a role. To evaluate the interference term, we need an expression for $E_{1,in}$ and $E_{2,in}$ in the cavity. To this end we use our knowledge that the cavity field has a node at the DBR on both sides of the cavity. The fields are thus given by:

$$E_{d,in} = |E_{d,in,max}|\left(\sin\left(\frac{2\pi n_d t_d}{\lambda_0}\right) + i\cos\left(\frac{2\pi n_d t_d}{\lambda_0}\right)\right) \tag{18}$$

$$E_{a,in} = |E_{a,in,max}|\left(-\sin\left(\frac{2\pi n_a t_a}{\lambda_0}\right) - i\cos\left(\frac{2\pi n_a t_a}{\lambda_0}\right)\right), \tag{19}$$

where the field in air travelling to the left has a $\pi$ phase flip compared to the field in diamond travelling to the right resulting from reflection off the mirror. $E_{d,in,max}$ and $E_{a,in,max}$ are the maxima of the incoming field in the diamond and air part respectively. They are related by Eq. 10 of the main text:

$$|E_{a,in,max}| = \sqrt{\frac{n_d}{n_a}}\sqrt{I_{rel}}|E_{d,in,max}|; \tag{20}$$
$$I_{rel} \equiv \frac{n_a}{n_d}\sin^2\left(\frac{2\pi n_d t_d}{\lambda_0}\right) + \frac{n_d}{n_a}\cos^2\left(\frac{2\pi n_d t_d}{\lambda_0}\right)$$

where we have defined the relative intensity as $I_{rel}$ to simplify the notation in further calculations.

Further, we know that the air gap width on-resonance is related to $t_d$ as given by eq. (8):

$$\frac{2\pi n_a t_a}{\lambda_0} = \arctan\left(-\frac{n_a}{n_d}\tan\left(\frac{2\pi n_d t_d}{\lambda_0}\right)\right), \tag{21}$$

where we keep $n_a = 1$ in the expression. such that:

$$\sin\left(\frac{2\pi n_a t_a}{\lambda_0}\right) = -\sqrt{\frac{1}{I_{rel}}}\sqrt{\frac{n_a}{n_d}}\sin\left(\frac{2\pi n_d t_d}{\lambda_0}\right); \tag{22}$$
$$\cos\left(\frac{2\pi n_a t_a}{\lambda_0}\right) = \sqrt{\frac{1}{I_{rel}}}\sqrt{\frac{n_d}{n_a}}\cos\left(\frac{2\pi n_d t_d}{\lambda_0}\right). \tag{23}$$

With eqs. (20), (22) and (23), we can rewrite the field in the air-part in terms of $|E_{d,in,max}|$ and $t_d$:

$$E_{a,in} = |E_{d,in,max}|\left(\sin\left(\frac{2\pi n_d t_d}{\lambda_0}\right) - i\frac{n_d}{n_a}\cos\left(\frac{2\pi n_d t_d}{\lambda_0}\right)\right). \tag{24}$$

We now have all the ingredients we need to evaluate the losses per cavity round trip. For that, we add the losses from the diamond side ($n_1 = n_d$) and from the air side ($n_2 = n_a$), weighting the last one by the factor comparing the relative intensities, as we have done before for the mirror losses. Using the expressions we found above, we arrive at the resulting expression:

$$\mathcal{L}_{S,\text{eff}} = \mathcal{L}_{S,DA} + \frac{n_a E^2_{max,a}}{n_d E^2_{max,d}}\mathcal{L}_{S,AD} \tag{25}$$
$$= 1 - \frac{|\rho'_{12}E_{d,in} + \tau'_{21}E_{a,in}|^2}{|E_{d,in}|^2} + I_{rel}\left(1 - \frac{|\rho'_{21}E_{a,in} + \tau'_{12}E_{d,in}|^2}{|E_{a,in}|^2}\right) \tag{26}$$
$$= 1 + I_{rel} - \frac{|\rho'_{12}E_{d,in} + \tau'_{21}E_{a,in}|^2 + \frac{n_a}{n_d}|\rho'_{21}E_{a,in} + \tau'_{12}E_{d,in}|^2}{|E_{d,in}|^2} \tag{27}$$
$$= 1 + I_{rel} - \left(\rho'^2_{12} + I_{rel}\frac{n_d}{n_a}\tau'^2_{21} + \frac{n_a}{n_d}I_{rel}\frac{n_d}{n_a}\rho'^2_{21} + \frac{n_a}{n_d}\tau'^2_{12}\right) \tag{28}$$
$$- \left(\rho'_{12}\tau'_{21} + \frac{n_a}{n_d}\rho'_{21}\tau'_{12}\right)\frac{E_{a,in}E^\star_{d,in} + E_{d,in}E^\star_{a,in}}{|E_{d,in}|^2} \tag{29}$$
$$\approx n_1\frac{(n_1-n_2)^2}{n_1+n_2}\left(\frac{4\pi\sigma_{DA}}{\lambda_0}\right)^2 + I_{rel}n_2\frac{(n_1-n_2)^2}{n_1+n_2}\left(\frac{4\pi\sigma_{DA}}{\lambda_0}\right)^2 \tag{30}$$
$$+ n_2\frac{(n_1-n_2)^2}{n_1+n_2}\left(\frac{4\pi\sigma_{DA}}{\lambda_0}\right)^2\left(2\sin^2\left(\frac{2\pi n_d t_d}{\lambda_0}\right) - 2\frac{n_1}{n_2}\cos^2\left(\frac{2\pi n_d t_d}{\lambda_0}\right)\right) \tag{31}$$
$$= \sin^2\left(\frac{2\pi n_d t_d}{\lambda_0}\right)\frac{(n_2+n_1)}{n_1}(n_2-n_1)^2\left(\frac{4\pi\sigma_{DA}}{\lambda_0}\right)^2. \tag{32}$$

From this expression we find that the effective losses are proportional to $\sin^2(2\pi n_d t_d/\lambda_0)$, which is the field intensity at the interface. The losses will thus be 0 for an air-like mode, and maximal for a diamond-like mode.

## IV. ANALYTIC SOLUTION OF A COUPLED GAUSSIAN BEAMS MODEL

This section describes the derivation of the analytic solution to a coupled Gaussian beams model as presented in the main text in Section II. We here outline the model and corresponding boundary conditions, and provide an analytic

solution. We assume the diamond surface to be planar in the first part of this section, which is close to a realistic situation. In the second part of this section we provide an analytic solution for a curved diamond surface, in which that mode volume may be decreased compared to the planar situation.

We employ the standard notation for a Gaussian beam [9]:

$$U(\boldsymbol{r}) = \frac{A_1}{q(z)} \exp\left(-ik\frac{\rho^2}{2q(z)}\right) \exp(-ikz) \tag{33}$$

$$= A_0 \frac{w_0}{W(z)} \exp\left(-\frac{\rho^2}{W^2(z)}\right) \exp\left(-ikz - ik\frac{\rho^2}{2R(z)} + i\zeta(z)\right); \tag{34}$$

$$W(z) = w_0\sqrt{1+\left(\frac{z}{z_0}\right)^2}; \tag{35}$$

$$R(z) = z\left(1+\left(\frac{z_0}{z}\right)^2\right); \tag{36}$$

$$\zeta(z) = \arctan\frac{z}{z_0}; \tag{37}$$

$$w_0 = \sqrt{\frac{\lambda_0 z_0}{n\pi}}. \tag{38}$$

where the complex beam parameter $q(z) = z + iz_0$ has been written as

$$\frac{1}{q(z)} = \frac{1}{R(z)} - i\frac{\lambda_0}{\pi n W^2(z)}, \tag{39}$$

to make the beam width $W(z)$ and the wave front curvature $R(z)$ explicit in the formulation. $\zeta(z)$ is the Guoy phase shift that occurs as a result of the deviation of the Gaussian beam from a planar wave, and we use $A_0 = A_1/(iz_0)$. Further, $\rho$ is the radial coordination, $z$ the coordinate along the beam and $k = \frac{2\pi}{\lambda_0}$ the wavenumber. The Gaussian beam is a solution for a bare plane-concave cavity, but to describe the field in a hybrid diamond-air cavity the two regions with different refractive-index regions have to be treated separately. This is evident when considering that the relation between the Gaussian beam parameters $w_0$ and $z_0$ is dependent on the refractive index in which the Gaussian beam lives (see eq. (38)). The wave front curvature $R$ and beam widths $W$ of these separate beams in diamond and air are described as [1]:

$$R_d(z) = z\left(1+\left(\frac{z_{0,d}}{z}\right)^2\right); \tag{40}$$

$$R_a(z) = (z-\Delta z_a)\left(1+\left(\frac{z_{0,a}}{z-\Delta z_a}\right)^2\right); \tag{41}$$

$$W_d(z) = w_{0,d}\sqrt{1+\left(\frac{z}{z_{0,d}}\right)^2}; \tag{42}$$

$$W_a(z) = w_{0,a}\sqrt{1+\left(\frac{z-\Delta z_a}{z_{0,a}}\right)^2}. \tag{43}$$

The subscript $a$ ($d$) is used for the Gaussian beam in air (diamond). The beam waist of the diamond beam is fixed to be on the plane mirror in the considered geometry, and the air beam waist is at distance $\Delta z_a$ from the plane mirror. This distance, together with the Rayleigh lengths of the diamond and air beams ($z_{0,a}$ and $z_{0,d}$) fix the full description of the Gaussian beams in the cavity. They follow from the boundary conditions imposed by the cavity dimensions. These boundary conditions can be found by considering the 'ABCD-matrix' that transforms the Gaussian beam parameters going from air (with $n = n_a$) to diamond (with $n = n_d$) [9]:

$$\begin{pmatrix} A & B \\ C & D \end{pmatrix} = \begin{pmatrix} 1 & 0 \\ 0 & n_a/n_d \end{pmatrix}. \tag{44}$$

Following the corresponding ABCD law for Gaussian beams we then find that the complex beam parameters in diamond and air ($q_d$ and $q_a$) are related by:

$$q_d = \frac{Aq_a + B}{Cq_a + D} = \frac{q_a}{n_a/n_d}. \tag{45}$$

This leads to the following conditions on the beam curvature and beam width at the interface:

$$n_d R_a(t_d) = n_a R_d(t_d); \tag{46}$$
$$W_a(t_d) = W_d(t_d), \tag{47}$$

that can be solved analytically to give [10]:

$$w_{0,a} = w_{0,d}, \qquad (\to z_{0,a}/n_a = z_{0,d}/n_d). \tag{48}$$
$$\Delta z_a = t_d\left(1 - \frac{n_a}{n_d}\right). \tag{49}$$

Together with the boundary condition that the beam front curvature follows the radius of curvature of the fiber dimple:

$$R_a(t_a + t_d) = ROC, \tag{50}$$

this gives an expression for the beam waist of the Gaussian beam:

$$w_{0,d} = w_{0,a} = \sqrt{\frac{\lambda_0}{\pi n_a}}\left(\left(t_a + \frac{t_d}{n_d}\right)\left(ROC - \left(t_a + \frac{t_d}{n_d}\right)\right)\right)^{1/4}. \tag{51}$$

In this expression we recognize the standard expression for the beam waist [11], with the cavity length replaced by:

$$L' \equiv t_a + \frac{t_d}{n_d} \; (= t_a + t_d - \Delta z_a). \tag{52}$$

The numerically and analytically obtained results to the model are both shown in fig. 4. We see that the stability condition for the cavity changes from the condition for a bare cavity. The stability condition of a cavity is found by requiring that the Rayleigh length satisfies $z_0^2 > 0$. For a bare cavity of length $L$ this gives, in combination with the boundary condition $R(L) = ROC$, the requirement $L < ROC$. The maximum cavity length is thus given by the radius of curvature of the concave mirror. But, for the hybrid cavity we see in fig. 4 that the cavity is stable beyond $t_d + t_a = ROC$, where $t_a = 16$ $\mu$m. For the hybrid cavity the beam waist of the air mode can be disconnected from the plane mirror such that we expect the cavity stability region to be given by $t_a + t_d - \Delta z_a$. Indeed, requiring $z_{0,a}^2 > 0$ in eq. (51) we find that the stability condition is:

$$t_a + \frac{t_d}{n_d} \lesssim ROC \tag{53}$$

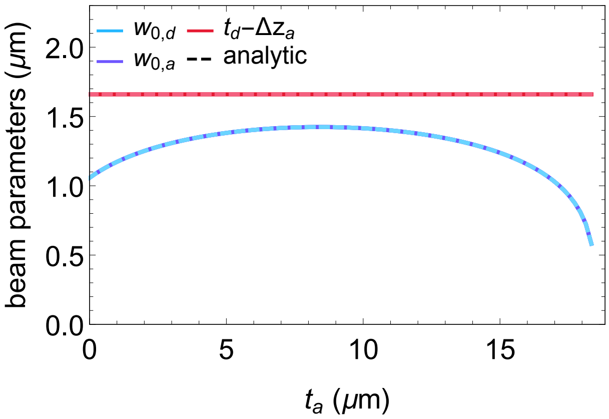


FIG. 4: The numerically calculated beam parameters (solid lines) versus the air gap of a diamond-air cavity with $t_d = 4$ $\mu$m and $ROC = 20$ $\mu$m. Analytically obtained results (eqs. (48), (49) and (51)) are shown as dashed lines. The analytical values for $w_{0,a}$ and $w_{0,d}$ overlap.

### Analytic solution for a curved diamond surface

We here derive the analytic solutions to the coupled Gaussian beams model if the diamond surface were curved, fixing the diamond surface radius of curvature to match the beam front curvature. While the diamond-air interface is more accurately described by a plane interface, the beam waist for a curved surface can be decreased for a curved diamond surface. This may produce a cavity with a smaller mode volume.

The ABCD matrix for this situation is given by:

$$\begin{pmatrix} A & B \\ C & D \end{pmatrix} = \begin{pmatrix} 1 & 0 \\ -\frac{(n_d - n_a)}{n_d R_{DA}} & n_a/n_d \end{pmatrix}, \tag{54}$$

where $R_{DA}$ is the radius of curvature of the diamond surface, that we assume to match the diamond and air Gaussian beam radius of curvature at that position: $R_a(t_d) = R_d(t_d) = -R_{DA}$. Following the ABCD-law, the complex beam parameters are related as:

$$q_d = \frac{Aq_a + B}{Cq_a + D} = \frac{q_a}{-\frac{(n_d - n_a)}{n_d R_{DA}} q_a - n_a/n_d}. \tag{55}$$

The boundary conditions that this leads to are:

$$R_a(t_d) = R_d(t_d); \tag{56}$$

$$W_a(t_d) = W_d(t_d), \tag{57}$$

that can be solved analytically to give:

$$z_{0,a} = \frac{n_d n_a (1 + t_d^2/z_{0,d}^2)}{n_d^2 + n_a^2 t_d^2 / z_{0,d}^2} z_{0,d} \approx \frac{n_a}{n_d} z_{0,d}, \qquad (\rightarrow w_{0,a} \approx w_{0,d}). \tag{58}$$

$$\Delta z_a = t_d \left( 1 - \frac{n_d^2 (1 + t_d^2/z_{0,d}^2)}{n_d^2 + n_a^2 t_d^2 / z_{0,d}^2} \right) \approx t_d \left(1 - n_a^2 n_d^2\right), \tag{59}$$

where the approximation holds in the case $t_d \ll z_{0,d}$, which holds in the case that $ROC \gg t_d$, as will be justified below. We find that the 'effective cavity length' that determines the beam waist for the case with such a curved surface is $L'_{curv} \approx t_a + t_d/n_d^2$. This length is shorter than for a plane diamond surface, since the surface curvature creates a lensing effect, shifting the effective waist position of the Gaussian beam in air towards the diamond-air interface. The shorter effective length gives a narrower beam waist compared to the plane diamond.

*a.* **Derivation of $\mathbf{t_d \ll z_{0,d}}$ for $\mathbf{ROC \gg t_d}$** In this paragraph we show that if we assume $ROC \gg t_d$, than it follows that $t_d \ll z_{0,d}$. First we assure ourselves that if $ROC \gg t_d$ holds, $R_{DA} \gg t_d$ also holds, where $R_{DA}$ is the beam curvature at the diamond-air interface. We can deduce this by finding the conditions for which $R_{DA} = ROC$, and then deducing that $R_{DA} > ROC$ for at least all cavities with $2t_d + t_a < ROC$. We do this as follows: first we find the two solutions of $R_a(z) = ROC$:

$$z - \Delta z_a = \frac{ROC}{2} \pm \frac{\sqrt{ROC^2 - 4z_{0,a}^2}}{2}$$

If $R_{DA} = ROC$, one of these solutions must correspond to $z = t_d$, while the other should correspond to $z = t_a + t_d$. We thus conclude that $t_a = \sqrt{ROC^2 - 4z_{0,a}^2}$. If we use this in the solution for $z = t_d$ we find: $t_d - \Delta z_a = ROC/2 - t_a/2$. This is the limiting case: to have $R_{DA} < ROC$ we require $t_d + t_a/2 - \Delta z_a < ROC/2$, or at least $2t_d + t_a < ROC$. This condition is almost always satisfied for cavities with $t_d \ll ROC$ since in that case the condition reduces to $t_a \lessapprox ROC$ which holds for all stable cavities.

We then use the constraint $t_d \ll R_{DA}$ to find constraints on $z_{0,d}$ and $z_{0,a}$. To this end we write $R_{DA}$ as $R_d(t_d)$ and $R_a(t_d)$ using eq. (40). $t_d \ll R_{DA}$ with $R_{DA} = R_d(t_d)$ respectively, gives:

$$t_d \ll t_d \left(1 + \frac{z_{0,d}}{t_d}\right)^2; \tag{60}$$

using $(t_d - \Delta z_a) < t_d \ll R_{DA}$ for the second equation. From this we find:

$$z_{0,d} \gg t_d; \tag{61}$$

## V. QUANTITATIVE ESTIMATES OF A MINIMUM AIR GAP WIDTH

The minimum air gap in a diamond-air cavity is civen by the geometry of the dimple. We here give a detailed description of the relevant parameters.

Independent of the fabrication procedure, the dimple depth $z_d$ is fixed by the radius of curvature and the useful dimple diameter $D_d$ as $z_d \approx D_d^2/(8ROC)$ [11]. For dimples with radii of curvature as considered in this manuscript ($\approx 15 - 35$ $\mu$m) and a diameter large enough to prevent clipping losses (see main text Section III B), $D_d \approx 8$ $\mu$m), the dimple depth is $z_d \approx 0.2 - 0.5$ $\mu$m. An extra air gap $z_f$ is introduced when there is an angle $\theta$ between optical fiber or plate in which the dimple is created and the flat substrate. If the extent beyond the dimple centre is $D_f/2$, the extra air gap is $z_f = \frac{D_f}{2}\sin(\theta) \approx \frac{D_f}{2}\theta$. For setups with an optical fiber on a tip-tilt stage [2], we estimate that the maximum angle the fiber tip makes with the flat substrate is $\theta_{max} \approx 70$ mrad ($\approx 20$ mrad from the tip-tilt stage and $\approx 50$ mrad from tilt due to mounting of the fiber). In combination with a typical fiber diameter of $D_f = 125$ $\mu$m, this leads to $z_{\mathrm{f,max}} \approx 4.4$ $\mu$m. This effect if thus dominant over the dimple depth. To reduce the minimal air gap in fiber-based cavities, the most important approach to lowering the mode volume is thus by shaping the fiber tip [12]. For cavities employing silica plates the large extent of the plates demands careful parallel mounting of the mirror substrates.

## VI. MODELLING THE EFFECT OF VIBRATIONS ON THE ZPL EMISSION

This section describes how the effect of vibrations is included in the model that describes the emission into the ZPL. First, we find the cavity resonance frequencies for length detuning $dt_a$, and use these to calculate the corresponding spectral overlap with the NV center emission frequency via

$$\xi_s(dt_a) = \frac{1}{1 + 4Q^2\left(\frac{\lambda_{\mathrm{ZPL}}}{\lambda_{\mathrm{cav}}(dt_a)} - 1\right)^2}, \tag{62}$$

where $\lambda_{\mathrm{ZPL}}$ is the NV emission frequency and $\lambda_{\mathrm{cav}}(dt_a)$ the cavity frequency for length detuning $dta$. $Q = \nu/\delta\nu$ is the cavity quality factor, that is calculated using the analytic methods presented in section II of the main text. We next multiply the Purcell factor found for the on-resonance case by the spectral overlap and calculate the resulting emission into the ZPL for each length detuning. Finally an average branching ratio $\beta_{\mathrm{vib}}$ is obtained by assuming that the cavity length is normally distributed around the resonant length with a standard deviation $\sigma_{\mathrm{vib}}$, and integrating over all air gaps around the resonance:

$$\beta_{\mathrm{vib}} = \int \frac{\beta_0 \xi_s(dt_a) F_p}{\beta_0 \xi_s(dt_a) F_p + 1} \frac{1}{\sqrt{2\pi\sigma_{\mathrm{vib}}^2}} \mathrm{e}^{-\frac{dt_a^2}{2\sigma_{\mathrm{vib}}^2}} \mathrm{d}(dt_a) \tag{63}$$

This integral is integrated numerically, to obtain the average branching ratio into the ZPL.

## VII. COUPLING EFFICIENCY OF A FIBER-BASED MICROCAVITY

In this section we describe the collection efficiency of the cavity mode, for a fiber-based microcavity. To that end we focus on how well the cavity mode can be matched to the detection mode. In our setup we have two possible detection routes: directly into the laser-machined fiber, or via the free-space path. On the side of the free space path the cavity mode can be overlapped with the mode of the collection path using free space elements. By optimal positioning of the optical elements the coupling can in principle have unit efficiency. On the fiber-side of the cavity path such flexibility is not present. The mode-matching efficiency is determined by the power transmittivity $\tau$ given by the overlap between the Gaussian beams in the fiber and the cavity mode [11, 13]:

$$\tau = \int U_f^*(\vec{r}) U_c(\vec{r}) d\vec{r}. \tag{64}$$

The Gaussian beams $U(\vec{r})$ are given by eq. (34) in the fiber and cavity, at $z = t_a + t_d$. The integral is over the radial direction. The relevant parameters are thus the beam widths and curvatures in the fiber ($w_f, R_f$) and cavity ($w_m, R_m = ROC$), as well as the spatial overlap of the beams given by the potential misalignment of the fiber due to an off-centred dimple and fiber tilt.

The resulting coupling efficiency (solid lines in fig. 5(a)) approaches unity for a large dimple radius of curvature if the beam width on the fiber mirror $w_m$ matches the beam radius in the fiber, $w_f = 2.5$ $\mu$m, providing the best overlap between the Gaussian beams. With the analytic model described in section III of the main text and section IV above, we can determine $w_m$ from the radius of curvature, size of the air gap and diamond thickness through eqs. (43), (48) and (51). Using this we determine what coupling parameter is achievable for our cavity parameters. Figure 5(b) shows that to achieve a coupling efficiency of $> 0.75$ an $ROC > 35$ $\mu$m in combination with an air gap $> 2$ $\mu$m is needed.

In addition spatial misalignment due to fiber tilt may significantly influence the coupling efficiency. If the fiber tilt is $\theta = 50$ mrad (fig. 5, dashed lines), a coupling efficiency $> 0.75$ can only be achieved for $ROC > 100$ $\mu$m. The influence of an off-centred dimple of $dx < 0.5$ $\mu$m is negligible.

The decrease of the coupling efficiency for smaller radius of curvature and air gap is in direct conflict with the maximalisation of the Purcell factor. To avoid having to trade-off these quantities, detection via the free space path is beneficial. A stability-argument can however be made for detection through the fiber: vibrations of the cavity as a whole with respect to the optical table, as resulting from passive vibration isolation used to minimize intra-cavity vibrations [2], might hinder free-space detection. Detection and (low-power, resonant) excitation through the fiber would remove the need to actively stabilize these vibrations.

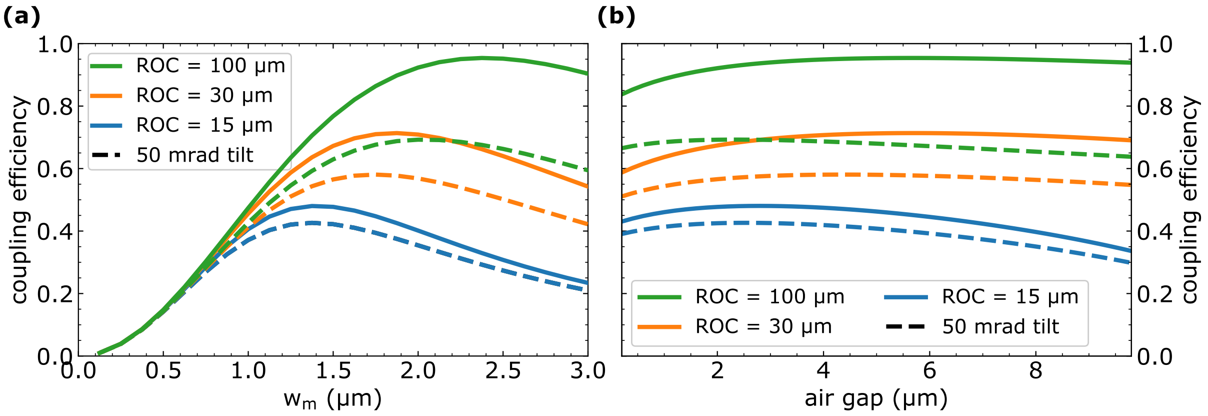


FIG. 5: (a) The mode matching efficiency into the dimpled fiber approaches unity for an ROC of 100 $\mu$m, if the beam width on the mirror approaches unity for an ROC of 100 $\mu$m, if the beam width on the mirror approached the beam width in the fiber ($w_f = 2.5$ $\mu$m). A fiber tilt of 50 mrad (dashed lines) decreases the maximally achievable coupling efficiency. (b) For $t_d = 4$ $\mu$m the air gap width should be $\gtrsim 2$ $\mu$m to maximize the coupling efficiency.


[1] E. Janitz, M. Ruf, M. Dimock, A. Bourassa, J. Sankey, and L. Childress, Phys. Rev. A **92**, 043844 (2015).
[2] S. Bogdanović, S. B. van Dam, C. Bonato, L. C. Coenen, A. M. J. Zwerver, B. Hensen, M. S. Liddy, T. Fink, A. Reiserer, M. Lončar, and R. Hanson, Appl. Phys. Lett. **110**, 171103 (2017).
[3] T. K. Yeung, D. Le Sage, L. M. Pham, P. L. Stanwix, and R. L. Walsworth, Appl. Phys. Lett. **100**, 251111 (2012).
[4] W. Pfaff, B. Hensen, H. Bernien, S. B. van Dam, M. S. Blok, T. H. Taminiau, M. J. Tiggelman, R. N. Schouten, M. Markham, D. J. Twitchen, and R. Hanson, Science **345**, 532 (2014).
[5] I. Filiński, Phys. Status Solidi B **49**, 577 (1972).
[6] J. Szczyrbwoski and A. Czapla, Thin Solid Films **46**, 127 (1977).
[7] C. C. Katsidis and D. I. Siapkas, Appl. Opt. **41**, 3978 (2002).
[8] S. J. Orfanidis, *Electromagnetic Waves and Antennas* (Rutgers University, Piscataway, NJ, 2002).
[9] B. Saleh and M. Teich, *Fundamentals of Photonics*, Wiley Series in Pure and Applied Optics (Wiley, 2007).
[10] S. Nemoto, Appl. Opt. **27**, 1833 (1988).
[11] D. Hunger, T. Steinmetz, Y. Colombe, C. Deutsch, T. W. Hänsch, and J. Reichel, New J. Phys. **12**, 065038 (2010).
[12] H. Kaupp, T. Hümmer, M. Mader, B. Schlederer, J. Benedikter, P. Haeusser, H. C. Chang, H. Fedder, T. W. Hänsch, and D. Hunger, Phys. Rev. Appl. **6**, 054010 (2016).
[13] W. B. Joyce and B. C. DeLoach, Appl. Opt. **23**, 4187 (1984).
